# Supplementary material for: SeaKR: Self-aware Knowledge Retrieval for Adaptive Retrieval Augmented Generation
Source: arXiv:2406.19215 source file (2024-06-27)
Supplement: Supplementary file 1 [file Appendix0_-_uncertainty-reranking.tex]

\begin{table}[]
\centering
\resizebox{\linewidth}{!}{
\setlength{\tabcolsep}{3.5pt}
\begin{tabular}{lrrrrrrrrrr}
\toprule
\multirow{2}{*}{Method} & \multicolumn{2}{c}{NQ} & \multicolumn{2}{c}{TriviaQA} & \multicolumn{2}{c}{SQuAD} \\
\cmidrule(r){2-3} \cmidrule(r){4-5} \cmidrule(r){6-7}
& 
\multicolumn{1}{c}{EM} & \multicolumn{1}{c}{F1} & \multicolumn{1}{c}{EM} & \multicolumn{1}{c}{F1} & \multicolumn{1}{c}{EM} & \multicolumn{1}{c}{F1} \\
\midrule
Prompt-Based & $23.4$&$33.4$ \\
% Judge-Then-Gen & \\
Perplexity & $22.5$ & $32.9$& $51.5$ & $59.9$\\
Energy & $21.7$  & $31.3$ & $51.8$ & $60.5$\\
LN Entropy & $25.1$ & $35.3$ & $53.1$ & $61.8$\\
\midrule
Eigen Score & $\mathbf{25.6}$ & $\mathbf{35.5}$ &$\mathbf{54.4}$ & $\mathbf{63.1}$\\
%llama2-7b-chat

\bottomrule
\end{tabular}
}
\caption{Comparison of other uncertainty measurement on reranking Top 10 documents.}
\label{tab:uncertainty-reranking}
\end{table}

% \model & -&-&0.356&0.4767&0.258&0.3003 \\ %llama3-8b-instruct

% \model & -&-&0.356&0.4767&0.258&0.3003 \\ %llama3-8b-instruct
