# Supplementary material for: SeaKR: Self-aware Knowledge Retrieval for Adaptive Retrieval Augmented Generation
Source: arXiv:2406.19215 source file (2024-06-27)
Supplement: Supplementary file 2 [file Appendix1-llama3-final-answer.tex]

\begin{table}[]
\centering
\scalebox{0.95}{
\setlength{\tabcolsep}{3pt}
\begin{tabular}{lrrrrrrrrrr}
\toprule
\multirow{2}{*}{Model} & \multicolumn{2}{c}{2Wiki} & \multicolumn{2}{c}{HotpotQA} & \multicolumn{2}{c}{IIRC} \\
\cmidrule(r){2-3} \cmidrule(r){4-5} \cmidrule(r){6-7}
& 
\multicolumn{1}{c}{EM} & \multicolumn{1}{c}{F1} & \multicolumn{1}{c}{EM} & \multicolumn{1}{c}{F1} & \multicolumn{1}{c}{EM} & \multicolumn{1}{c}{F1} \\
\midrule
Final Step & $40.9$ & $47.5$ & $34.6$ & $46.6$ &$\textbf{26.6}$&$\textbf{30.7}$\\
CoT Reader & $40.2$ & $46.7$ & $35.2$ & $47.0$ &$25.8$&$30.0$\\
Adaptive & $\textbf{41.1}$ & $\textbf{47.8}$ & $\textbf{35.6}$ & $\textbf{47.7}$ & $25.8$ & $30.0$ \\
\bottomrule
\end{tabular}
}
\caption{Comparison of different final answer aggregation strategies in multihop reasoning. "Final Step" strategy extracts the answer directly from the final step generated. CoT Reader uses a posthoc CoT Reader that takes all retrieved passages and the query, generating new CoT steps and an answer. The "Adaptive" strategy adaptively chooses either method based on their average eigen score across different steps.}
\label{tab:synthesis}
\end{table}

% \model & -&-&0.356&0.4767&0.258&0.3003 \\ %llama3-8b-instruct
